# Supplementary material for: Sharp Integrality Gaps in Calibration Distance
Source: arXiv:2610.05679 source file (2026-10-05)
Supplement: Supplementary file 1 [file joint_lower_family_supplement.tex]

% Supplementary proof accompanying the manuscript.
% It is not required for the joint upper-bound theorem in the main text.
\section{Endpoint Padding and a Stronger Joint Lower Family}
\label{app:joint-lower-family-supplement}

\begin{lemma}[Endpoint padding invariance]
Appending any number of $(x,p)=(0,0)$ identities leaves both $\CalDist$
and $\LowerCalDist$ unchanged.  The analogous statement holds for
$(x,p)=(1,1)$.
\end{lemma}
\begin{proof}
The zero-cost extension gives one inequality.  For the reverse deterministic
inequality, a padded group with $R$ original records, $Z$ appended zeros,
and $u$ positive labels has destination $q=u/(R+Z)$.  If $R>0$, move the
original records to $q_0=u/R$; the cost increase is at most
$R(q_0-q)=Zq$, exactly the removed padding cost.  Groups with $R=0$ are
deleted.  For a finite fractional repair, write $R_q,Z_q,U_q$ for the
original mass, padding mass and positive mass at $q$.  Calibration gives
$U_q=q(R_q+Z_q)$.  Move original mass to $U_q/R_q$ when $R_q>0$; the
increase is at most $qZ_q$.  Merging destinations preserves every source
row and gives residual
$\sum(U_q-\alpha R_q)=0$ at each new destination $\alpha$.  Taking
infima and complementing labels proves the claim.
\end{proof}

\begin{theorem}[A stronger joint lower family]
For integers $k\geq6$, $h,R\geq1$, let
\[
 \mathcal F_k=\{a/b:0<a<b\leq k,\ \gcd(a,b)=1,\ b>k/2\},
 \quad K=|\mathcal F_k|,\quad B_c=\sum_{a/b\in\mathcal F_k}b.
\]
There is a rational binary unit input with
\[
 T_0=\frac{2RB_c(8^h-1)}7,\qquad m_0=2Kh,
\]
for which
\begin{equation}
 \CalDist=\frac{hB_c}{32k^2},\qquad
 \LowerCalDist\leq\frac{B_c(1-8^{-h})}{896k^4R},\qquad
 \CalDist-\LowerCalDist\geq\frac{kh}{5000}.
 \label{eq:joint-lower-family-supplement}
\end{equation}
The construction can be padded to every $T\geq T_0$ with at most $m_0+1$
original forecast values and the same gap.
\end{theorem}
\begin{proof}
For $c=a/b\in\mathcal F_k$ and $j<h$, set
$n_{c,j}=Rb8^j$ and $e_j=(64k^2R8^j)^{-1}$.  At each of
$c-e_j,c+e_j$ place $n_{c,j}$ identities, with $Ra8^j$ ones and
$R(b-a)8^j$ zeros.  Centers are at least $k^{-2}$ apart and
$e_j\leq E=(64k^2R)^{-1}$, so the forecasts are distinct and lie in
$(0,1)$.  The count gives $T_0,m_0$.

Price an original record by $e_j$ and padding by zero.  For a center,
if $M_c(s)$ counts records with $e_j>s$, then
\[
 sM_c(s)<\frac{b}{28k^2}\leq\frac1{28b}<\frac1{12b}.
\]
For a calibrated group of size $N$ and mean $q=u/N$, if all centers are
at distance at least $2E$, every original record pays at least its price.
Otherwise a unique $c=a/b$ has $d=|q-c|<2E$.  If $d>0$, then
$d\geq1/(bN)$.  Only records from this center with $e_j>d/4$ are counted
in $g$; the tail bound gives $g\leq1/(3bd)\leq N/3$.  These records pay
at least $e_j-d$, all other original records pay at least $e_j+d/2$, and
records from other centers satisfy the same bound because
$2e_j+3d/2<5E<k^{-2}$.  Padding records pay at least $d/2$.  Thus
\[
 \sum_{t\in G}|p_t-q|
 \geq\sum_{t\in G}e_t-dg+\frac d2(N-g)
 =\sum_{t\in G}e_t+\frac d2(N-3g)
 \geq\sum_{t\in G}e_t.
\]
Sending each center to itself and padding to zero attains the price sum,
so $\CalDist=hB_c/(32k^2)$.

For the fractional witness, exchange mass
$n_{c,j}e_j=b/(64k^2)$ from a positive left record to the right and the
same mass from a zero right record to the left.  The destination masses
and means remain $n_{c,j}$ and $c-e_j,c+e_j$; the cost is
$4n_{c,j}e_j^2$ per scale.  Summation gives the displayed upper bound on
$\LowerCalDist$.  Coprime-pair counting gives $K\geq k^2/72$ and
$B_c\geq k^3/144$, so the gap exceeds $kh/5000$.  Padding preserves it
by the lemma.  Taking $R=1$ gives the sufficient conditions
$k^2h+1\leq m$ and $k^3(8^h-1)/7\leq T$.
\end{proof}

For $R=1$ and $h=\lceil\log_8k\rceil$, this family has
$T_0=\Theta(k^4)$, $m_0=\Theta(k^2\log k)$ and gap order $k\log k$.
It is a lower family, not a characterization of the exact joint order.
